# Supplementary material for: Statistical Learning under Heterogeneous Distribution Shift
Source: arXiv:2302.13934 source file (2023-10-27)
Supplement: Supplementary file 1 [file sum_reg_proofs.tex]

%!TEX root = ../main.tex

\section{Proofs}

\section{Proofs}

\begin{proof}[Proof of \Cref{lem:talagrand_ap}] Handling $G_n[\cC]$ requires truncation. 
Define $\bar{\xi}_i := \xi_i \I\{|\xi_i| \le \sqrt{2\log(6n/\delta)}\}$, and set
\begin{align*}
\bar{G}_n[\cC] := \sup_{(f,\upbeta) \in \Pif \cC}\frac{1}{n}\sum_{i=1}^n \bar \xi_i (f-\fst - \upbeta)(X_i)
\end{align*}
Applying \Cref{lem:talagrand}, with probability $1 - \delta/3$, using that $|\bar \xi_i (f-\fst - \upbeta)| \le B \sqrt{2\log(6n/\delta)}$ and by $(r,r_0)$-localization,
\begin{align*}
\Ezero[(\bar \xi_i(f-\fst - \upbeta)^2] = \Ezero[|\bar{\xi}|^2]\cdot \Ezero[(f-\fst - \upbeta)^2] \le r^2,
\end{align*}
we find that with probability $1-\delta/3$, 
\begin{align*}
\bar{G}_n[\cC]\le 2\Exp[\bar{G}_n[\cC]] + \sqrt{\frac{2r^2\log(1/\delta)}{n}} + \frac{4\sqrt{2\log(2n/\delta)}\log(3/\delta))B}{n}
\end{align*}
Moreover, with probability $1 - \delta/3$, it holds that$T_2[\cH_0] = \bar T_2[\cH_0]$. In addition, we have
\begin{align*}
|\Ezero[\bar{G}_n[\cH_0] - G_n[\cH_0]]| &\le \Ezero\sup_{(f,\upbeta) \in \Pif \cC} \sum_{i=1}^n|f-\fst - \upbeta_g)|\cdot |\xi_i-  \bar{\xi}_i| \\
&\le B \Exp_{\xi \sim \cN(0,1)}[|\xi| \I\{\xi \ge \sqrt{2\log(6n/\delta)}\}]\\
&= 2B \int_{\sqrt{2\log(6n^2/\delta)}}^{\infty} \frac{u e^{-u^2/2}}{\sqrt{2\pi}}du\\
&= 2B \sqrt{\frac{2}{\pi}} e^{-2\log(6n/\delta)} =  2B \sqrt{\frac{2}{\pi}} \frac{\delta^2}{36 n^2} \le B/18n^2. 
\end{align*}
Combing all three estimates shows the bound of \Cref{eq:some_bound_one} with probability $1-2\delta/3$. The estimate for $E_n$ is a direct consequence of \Cref{lem:talagrand}.
\end{proof}

\begin{proof}[Proof of \Cref{lem:symm_one}] Recall that 
\begin{align*}
\Ezero[E_n(\cC)] = \Ezero\left[\sup_{(f,g,\upbeta) \in \cC} \sum_{i=1}^n (f - \fst - \upbeta)(\gst - \upbeta - g)\right]
\end{align*}
First, consider $\cC \subset \ccf$. Let $X_{1:N}'$ be a random variables such that $X_i,X_i' \mid Y_i$ are i.i.d. Then, 
\begin{align*}
n\Ezero[E_n(\cC)] &= \Ezero\left[\sup_{(f,g,\upbeta) \in \cC} \sum_{i=1}^n (f - \fst - \Ezero[f - \fst \mid Y_i])(\gst - \upbeta - g)\right]\\
&= \Ezero\left[\sup_{(f,g,\upbeta) \in \cC} \sum_{i=1}^n (f(X_i) - \fst(X_i) - \Exp[f(X_i) - \fst(X_i) \mid Y_i])(\gst - \upbeta - g) \right]\\
&= \Ezero\left[\sup_{(f,g,\upbeta) \in \cC} \sum_{i=1}^n (f(X_i) - \fst(X_i) - \Exp[f(X_i') - \fst(X_i') \mid Y_i])(\gst - \upbeta - g) \right]\\
 &= \Ezero\sup_{(f,g,\upbeta) \in \cC} \Ezero\left[\sum_{i=1}^n (f(X_i) - \fst(X_i) - f(X_i') - \fst(X_i'))(\gst - \upbeta - g) \mid Y_{1:n},X_{1:n} \right]\\
 &\le \Ezero\sup_{(f,g,\upbeta) \in \cC} \left[\sum_{i=1}^n (f(X_i) - \fst(X_i) - (f(X_i') - \fst(X_i')))(\gst - \upbeta - g)  \right]\\
 &\le \Ezero\Ezero\sup_{(f,g,\upbeta) \in \cC} \left[\sum_{i=1}^n (f(X_i) - \fst(X_i) - (f(X_i') - \fst(X_i')))(\gst - \upbeta - g)  \mid Y_{1:n}\right]
\end{align*}
Observe that, for $(f,g,\upbeta) \in \cC \subset \ccf$, $\upbeta$ and $g$ are functions $Y$. Hence, conditioned on $Y_{1:n}$, $(f(X_i) - \fst(X_i) - (f(X_i') - \fst(X_i'))$ are symmetric random variables, so that 
\begin{align*}
&\Ezero\Ezero\sup_{(f,g,\upbeta) \in \cC} \left[\sum_{i=1}^n (f(X_i) - \fst(X_i) - (f(X_i') - \fst(X_i')))(\gst - \upbeta - g)  \mid Y_{1:n}\right] \\
&= \Ezero\Ezero\sup_{(f,g,\upbeta) \in \cC} \left[\sum_{i=1}^n \epsilon_i (f(X_i) - \fst(X_i) - (f(X_i') - \fst(X_i')))(\gst - \upbeta - g)  \mid Y_{1:n}\right]\\
&= \Ezero\Ezero\sup_{(f,g,\upbeta) \in \cC} \left[\sum_{i=1}^n \epsilon_i (f(X_i) - \fst(X_i) - \upbeta -  (f(X_i') - \fst(X_i') - \upbeta))(\gst - \upbeta - g)  \mid Y_{1:n}\right]\\
&= \Ezero\Ezero\sup_{(f,g,\upbeta) \in \cC} \left[\sum_{i=1}^n \epsilon_i (f(X_i) - \fst(X_i) - \upbeta -  (f(X_i') - \fst(X_i') - \upbeta))(g-\gst + \upbeta )  \mid Y_{1:n}\right]\\
&= 2\Ezero\left[\sup_{(f,g,\upbeta) \in \cC} \sum_{i=1}^n \epsilon_i (f(X_i) - \fst(X_i) - \upbeta) (g- \gst +\upbeta  )\right] \\
&= 2n\bar E_n(\cC)
\end{align*}
The symmetrization of $\cC \subset \ccg$ is specular.
\end{proof}
