# Supplementary material for: Statistical Learning under Heterogeneous Distribution Shift
Source: arXiv:2302.13934 source file (2023-10-27)
Supplement: Supplementary file 2 [file beyond_uniform.tex]

%!TEX root = ../icml_main.tex
